# Supplementary material for: Gaining Insights into Unrecognized User Utterances in Task-Oriented Dialog Systems
Source: arXiv:2204.05158 source file (2022-10-24)
Supplement: Supplementary file 1 [file 9-appendices.tex]

\appendix
\section{Appendices}
\subsection{Raduis-based Clustering Algorithm}
\label{sec:appendix-a}

\SetKwInOut{Input}{input}
\SetKwInOut{Output}{output}
\SetKwComment{Comment}{/*}{*/}

\begin{algorithm}
\caption{Radius-based Clustering}
\label{alg:clustering}
\SetInd{0.75em}{0.25em}
\small

\textbf{input}: {E (e1, e2, ... en)} \Comment{\hspace{0.05cm} elements}
%\textbf{input}: {D (n{$\times$}n)} \Comment{\hspace{0.05cm} dist matrix}
\textbf{input}: {min\_sim} \Comment{\hspace{0.05cm} min similarity}
\textbf{input}: {min\_size} \Comment{\hspace{0.05cm} min cluster size}
\BlankLine

$C \gets \emptyset$

\While{convergence criteria are not met}{
    \BlankLine
    \For{each element $e_i{\in}E$} {
        \BlankLine
        \eIf{the highest similarity of $e_i$ to any existing cluster exceeds min\_sim}{
            \BlankLine
            assign $e_i$ to its most similar cluster $c$ \\
            re-calculate the centroid of $c$
            \BlankLine
        }{
            \BlankLine
            create a new cluster $c^\prime$ and assign $e_i$ to it \\
            set the centroid of $c^\prime$ to be $e_i$ \\
            add $c^\prime$ to $C$
            \BlankLine
            
        }
    }
}
\BlankLine
\Comment{clusters with fewer elements than the predefined $min\_size$ are considered outliers}
\BlankLine
\textbf{return}: each $c{\in}C$ of size exceeding $min\_size$

\end{algorithm}

\subsection{Keyword-based Merging}
\label{sec:appendix-b}

%\paragraph{Keyword-based Merging}
User requests to a goal-oriented dialog system are likely to be characterized by the extensive use of a domain-specific lexicon. For example, in the domain of banking, we are likely to encounter terms related to `accounts', `transactions', and `balance', while in the context of a Covid-19 Q\&A bot, the lexicon is likely to contain extensive use of words related to `vaccine', `boosters', `appointments', and so on. Although impressive at capturing meaning, semantic representations do not necessarily capture the domain-specific notion of similar requests. For example, the two utterances `covid 19 and pregnancy' and `7 months pregnant and tested positive for covid, any risks?' do not exhibit exceptional semantic similarity, while practically they should be clustered together. The intuition that stems from the fact that both sentences contain `pregnant'/`pregnancy', and `covid' -- words typical of the underlying domain. We therefore suggest the additional, keyword-based merging approach, as detailed below.

%\paragraph{Domain-specific Keywords Extraction} 
A common way to extract lexical characteristics of a corpus is using a \textit{log-odds ratio with informative Dirichlet prior} \citep{monroe2008fightin} -- a method that discovers markers with excessive frequency in one dataset compared to another. We used the collection of unhandled utterances as our target corpus and a random sample of $100$K sentences from a Wikipedia dump\footnote{We used the Wikipedia 2006 dump available at \url{https://nlp.lsi.upc.edu/wikicorpus/}.} as our background neutral dataset. Setting the strict log-odds score of \text{-}$5$, markers identified for the dataset of Covid-19 requests included \{`quarantine', `measures', `emergency', `pregnant', `sick', `leave', `risk'\}.

%\paragraph{Cluster Similarity Computation} 
Given a set of markers, we now define cluster similarity as follows: we denote the set of domain-specific markers discovered by the log-odds ratio procedure by ${M}$ and the set of top-k most frequent words\footnote{k=$10$ by qualitative evaluation over the $[3, 15]$ range.} in two clusters $c_1$ and $c_2$, by ${W}_1$ and ${W}_2$, respectively. The similarity of $c_1$ and $c_2$ is then defined to be proportional to the number of markers from ${M}$ that can be found in both ${W}_1$ and ${W}_2$: $sim(c_1, c_2) \propto |{M} \cap {W}_1 \cap {W}_2|$, where $|{M}|$ amounts to the maximal possible similarity. Pairwise cluster distances are further computed by normalizing the similarity values to the $[0, 1]$ range, and subtracting them from $1$. A distance matrix $D_c$ is constructed by calculating pairwise distance on the set of clusters in ${C}$, and is further used as an input to a subsequent invocation of the RBC algorithm, with an adjusted \textit{min\_sim} threshold.

Following this definition and assuming a sample set of domain-specific markers \{`covid', `risk', `quarantine', `pregnant', `appointment', `test', `positive'\}, the two utterances `covid 19 and pregnancy' and `7 months pregnant and tested positive for covid, any risks?' will exhibit considerable keyword-based similarity (intersection size{=}2), despite only moderate semantic proximity.
